# Supplementary material for: Ranking Significant Discrepancies in Clinical Reports
Source: arXiv:2001.06674 source file (2020-01-18)
Supplement: Supplementary file 1 [file appendix.tex]

\clearpage
\section*{Appendix}

\subsection*{Model parameters}
We train each model for 20 epochs with a batch size of 16 and a learning rate of $10^{-3}$. This is adequate for model convergence. We use a 2-layer perceptron with sigmod activation for score combination. The hidden layer consists of 10 nodes. We initialize the weights with a normal distribution $\mathcal{N}(1,0.01)$. We initialize the unigram and n-gram term weights from $\mathcal{N}(0,0.01)$ with a bias of 1.

Through hyper-parameter tuning on the validation set, we found the following parameters to be optimal:
\begin{itemize}
\item N-grams: term bi-grams and tri-grams (tested no n-grams through 5-grams).
\item Word representations: SciBERT (base, uncased) layer 9 (tested BERT (base, uncased) and SciBERT (base, uncased), all layers)
\item SciBERT learning rate: $2\times 10^{-5}$ (tested $5\times 10^{-5}$, $3\times 10^{-5}$, and $2\times 10^{-5}$, as suggested by~\cite{Devlin2018BERTPO})
\end{itemize}

See \citet{Dehghani2017NeuralRM} for details about pairwise cross-entropy loss. Training pairs were randomly selected, such that the ``relevant'' pair has a higher degree of discrepancy than the ``non-relevant'' pair.
